# Supplementary material for: Enhancing Weakly Supervised Video Grounding via Diverse Inference Strategies for Boundary and Prediction Selection
Source: arXiv:2503.23181 source file (2025-03-29)
Supplement: Supplementary file 1 [file 7-supplementary.tex]

\clearpage

\section*{\centering
{ \LARGE Supplementary Material:} \\
Gaussian Mixture Proposals with Pull-Push Learning Scheme to Capture Diverse Events for Weakly Supervised Temporal Video Grounding}

\appendix 

% \tableofcontents

% \vfill\eject

\setcounter{equation}{10}
\setcounter{table}{5}
\setcounter{figure}{5}

%% Overview %%%%%%%%%%%%%%%%%%%%%%%%%%%%%%
\section{Overview}
\label{supp-sec:overview}
%%%%%%%%%%%%%%%%%%%%%%%%%%%%%%%%%%%%%%%%%%%%%%%%%%%%%%%%%%%%%
In this supplementary material, we first describe a potential negative societal impact we have to be aware of.
Second, we explain the details of datasets including the approval status from an Institutional Review Board (IRB).
Third, we describe more implementation details of our Pull-Push Scheme (PPS).
Fourth, we explain how we implement variants used for ablation studies.
Fifth, we show additional quantitative and qualitative results.
Lastly, we describe the information on the implemented code.
Additionally, we provide the implemented code of our PPS in the \path{code} folder from the supplementary material ZIP file.
% Additionally, we provide the implemented code and saved models of PPS in the \path{code} folder from the supplementary material ZIP file.

For convenience, the sections, equations, figures, and tables of the supplementary material follow those of the submitted paper.
On the other hand, the references of the supplementary material are separated from the references of the submitted paper.

%% Potential negative societal impact %%%%%%%%%%%%%%%%%%%%%%%%%%%%%%
\section{Potential Negative Societal Impact}
\label{supp-sec:potential-negative-societal-impact }
%%%%%%%%%%%%%%%%%%%%%%%%%%%%%%%%%%%%%%%%%%%%%%%%%%%%%%%%%%%%%
Since this algorithm can automatically retrieve temporal video locations corresponding to given sentences, it can be misused by malicious entities for the purpose of controlling people.
For instance, videos on social media and video-sharing sites can be automatically censored to restrict the liberty of people and suppress free speech.
To mitigate the risk, we will take responsibility for making this algorithm used only for research or social contribution by trustworthy individuals or organizations.

%% Details of datasets and approval status from an IRB %%%%%%%%%%%%%%%%%%%%%%%%%%%%%%
\section{Details of Datasets and IRB Approval Status}
\label{supp-sec:datasets}
%%%%%%%%%%%%%%%%%%%%%%%%%%%%%%%%%%%%%%%%%%%%%%%%%%%%%%%%%%%%%

%% ActivityNet Captions Dataset %%%%%%%%%%%%%%%%%%%%%%%%%%%%%%
\subsection{ActivityNet Captions}
The ActivityNet Captions dataset~\cite{krishna2017dense} has been widely used for dense video captioning and temporal video grounding, which contains 20,000 videos with 100,000 sentence queries.
In the ActivityNet Captions dataset, 10,009, 4,917, and 5,044 videos are given for training, validation, and testing, respectively.
The average lengths of the videos and the sentences are 120 seconds and 14 words, respectively.
Furthermore, there are 3.65 annotated locations in the video on average.
We don't exploit annotations of temporal locations during training for weakly supervised learning.
Since a testing set is not publicly available, we use $val_2$ for testing, which is the same data splitting strategy in~\cite{zhang2019cross} and other compared methods.

\paragraph{Approval from an Institutional Review Board (IRB).}
We have confirmed that the ActivityNet Captions dataset is approved by the Stanford IRB.

%% Charades-STA Dataset %%%%%%%%%%%%%%%%%%%%%%%%%%%%%%
\subsection{Charades-STA}
\cite{gao2017tall} makes a Charades-STA dataset from a Charades dataset~\cite{sigurdsson2016hollywood}, which is originally used for action recognition and video captioning, to extend the dataset to temporal video grounding.
The average lengths of the videos and annotated locations are 30 seconds and 8 seconds, respectively. 
Moreover, there are 2.4 annotated locations in the video on average.
We don't exploit annotations of temporal locations during training for weakly supervised learning.

\paragraph{Approval from an Institutional Review Board (IRB).}
It is unclear if the original Charades dataset is approved by an IRB.
However, it has not been withdrawn and is still offered by its creators.
Further, it is a widely used public dataset for many tasks such as action recognition, video captioning, and video grounding.
Especially, for fair comparisons with other weakly supervised temporal video grounding methods~\cite{lin2020weakly, ma2020vlanet, huang2021cross, zheng2022cpl, Chen_Luo_Zhang_Ma_2022, wang2021visual}, we need to evaluate the proposed methods on this dataset.

%% More implementation details %%%%%%%%%%%%%%%%%%%%%%%%%%%%%%
\section{More Implementation Details}
\label{supp-sec:more-implementation-details}
%%%%%%%%%%%%%%%%%%%%%%%%%%%%%%%%%%%%%%%%%%%%%%%%%%%%%%%%%%%%%

\subsection{Video encoder}
For video encoding, video segments of 16 frames are sampled from a video, which are overlapped with adjacent segments by half the segment length.
Then, $T$ evenly sampled video segments are obtained.
If the number of segments is less than $T$ due to a short input video, empty segments are filled with zero values.
We extract segment features from the $T$ segments of a video via 3D CNN-based feature extractors:
C3D~\cite{tran2015learning}
\footnote{{http://activity-net.org/challenges/2016/download.html\#c3d}.} for the ActivityNet Captions dataset and I3D~\cite{carreira2017quo}
\footnote{{https://github.com/piergiaj/pytorch-i3d}.} for the Charades-STA dataset.
The C3D and the I3D are pre-trained on sport1M~\cite{karpathy2014large} and Kinetics~\cite{carreira2017quo} datasets for feature extraction, respectively.
The extractors have a temporal resolution of 16 frames and features are extracted every 8 frames.
In the C3D, Principal Component Analysis (PCA) is used to reduce the feature dimension from the second fully connected layer (\ie from 4096 to 500 dimensions).
In the I3D, features whose dimension is 1024 are obtained via fully connected layers.

\subsection{Query encoder}
In query encoding, the sentence query which has more than 20 words is truncated to 20 words.
Then, we convert each word of the query to a lowercase letter and use the pre-trained GloVe~\cite{pennington2014glove} as word embeddings.
For positional information of words, the sinusoidal positional encoding vector~\cite{vaswani2017attention} is added to word features.
For the hidden sentence query, we randomly hide the original sentence query by replacing a third ($1/3$) of the words with [HIDE] tokens, same as the [MASK] tokens in \cite{devlin2018bert}.
Then, the equivalent query encoding is applied to the hidden sentence query to extract a hidden sentence query feature.

\subsection{Query reconstruction}
Here, we explain how to produce the reconstructed query and cross-entropy loss in the reconstruction.
Following other reconstruction-based methods~\cite{lin2020weakly,zheng2022cnm,zheng2022cpl}, for the query reconstruction, we calculate $\mathbf{R}^\mathbf{P}$ by replacing $\mathbf{M}$ with $\mathbf{P}\in\{\mathbf{P}_{p}, \mathbf{P}_{hn}, \mathbf{P}_{en}\}$ in Eq.~({8}) 
Then, $\mathbf{R}^\mathbf{P}$ is applied to a fully connected layer followed by a Softmax function to calculate
\begin{equation}
\mathbf{Z}^\mathbf{P}=\mathrm{Softmax}\left(\mathbf{W}_{\mathbf{Z}}\mathbf{R}^\mathbf{P}+\mathbf{b}_{\mathbf{Z}}\right), \mathbf{Z}^\mathbf{P} \in \mathbb{R}^{N\times B} \text{,}
  \label{supp-eq:softmax-masked-multi-modal-feature}
\end{equation}
where $\mathbf{W}_{\mathbf{Z}}$ and $\mathbf{b}_{\mathbf{Z}}$ are defined as learnable parameters of a fully connected layer, and $B$ is the vocabulary size.
The $(i,j)^{th}$ element of $\mathbf{Z}^\mathbf{P}$ denotes the probability of predicting the $j^{th}$ vocabulary word $\widetilde{w}_j$ for the $i^{th}$ word in the sentence query as follows: 
\begin{equation}
  Pr(\widetilde{w}_j|\mathbf{V},\widehat{\mathbf{Q}}_{0:i-1},\mathbf{P})=\mathbf{Z}^\mathbf{P}(i,j) \text{,}
  \label{supp-eq:prob-word}
\end{equation}
where
$\widehat{\mathbf{Q}}_{0:i-1}$ denotes the randomly hidden query features from the [START] token to the $(i$-$1)^{th}$ word.
Then, we use the cross-entropy loss $C(\cdot)$ to reflect the difference between the reconstructed query and the original query $\mathcal{S} = \{w_n\}_{n=1}^N$, which can be computed by
\begin{equation}
  C\left(\mathbf{P}\right)=-\sum _{n=1}^N \textrm{log}Pr\left(w_n|\mathbf{V},\widehat{\mathbf{Q}}_{0:n-1},\mathbf{P}\right) \text{.}
  \label{supp-eq:cross-entropy-loss}
\end{equation}

\subsection{Inference strategies}
Here, we explain the proposed inference strategies.
To predict temporal locations from Gaussian mixture proposals, we propose three inference strategies, which are 1) tail-to-tail, 2) average, and 3) importance-based inference.
First, we calculate left $\mathbf{t}$ and right $\mathbf{e}$ points for the selected proposal $\mathbf{P}_{p}^{(k^\dagger)}$ by
\begin{align}
  &\mathbf{t}=\mathbf{c}^{(k^\dagger)}-\gamma\mathbf{s}^{(k^\dagger)}/2\in \mathbb{R}^{E_p} \text{,}  
  \label{supp-eq:start}\\
  &\mathbf{e}=\mathbf{c}^{(k^\dagger)}+\gamma\mathbf{s}^{(k^\dagger)}/2\in \mathbb{R}^{E_p} \text{,}
  \label{supp-eq:end}
\end{align}
where $k^\dagger$ is the index of the selected proposal by vote-based selection~\cite{zhou2021ensemble, zheng2022cpl}, $\gamma$ is a hyper-parameter to control the widths of predicted temporal locations, and $E_p$ is the number of masks in the positive proposal.
The tail-to-tail-based inference predicts normalized temporal locations starting at $o_{s}$ and ending at $o_{e}$ by selecting the points on the far left and the far right.
\begin{align}
  &o_{s} = \mathrm{max} \left(\mathrm{min}_l\,\mathbf{t}_l,0\right) \in\mathbb{R}\text{,} \\
  &o_{e} = \mathrm{min} \left(\mathrm{max}_l\,\mathbf{e}_l,1\right) \in\mathbb{R}\text{,}
  \label{supp-eq:minmax-inference}
\end{align}
where $\mathbf{t}_l$ and $\mathbf{e}_l$ are the $l^{th}$ elements of $\mathbf{t}$ and $\mathbf{e}$, respectively.
The average-based inference predicts normalized temporal locations by averaging the left points and the right points.
\begin{align}
  &o_{s} = \mathrm{max} \biggl(\frac{1}{E_p}\sum_{l=1}^{E_p}\mathbf{t}_{l},0\biggl) \in\mathbb{R}\text{,}  \\
  &o_{e} = \mathrm{min} \biggl(\frac{1}{E_p}\sum_{l=1}^{E_p}\mathbf{e}_{l},1\biggl) \in\mathbb{R}\text{.}
  \label{supp-eq:average-inference}
\end{align}
In the importance-based inference, normalized temporal locations are obtained by pooling the left points and the right points with the importance weights $\mathbf{w}^{(k^\dagger)}$ in Eq.~({10}), as
\begin{align}
 &o_{s} = \mathrm{max} (\mathbf{w}^{(k^\dagger)\top}\mathbf{t},0) \in \mathbb{R} \text{,}  \\
 &o_{e} = \mathrm{min} (\mathbf{w}^{(k^\dagger)\top}\mathbf{e},1) \in \mathbb{R}\text{.} 
 \label{supp-eq:importance-inference}
\end{align}
For the final predicted temporal locations, we multiply the normalized temporal locations by the length of a given video.
The impact of different inference strategies is studied in \cref{supp-tab:ablation-inference}.

\subsection{Other details}
The proposed scheme, PPS, was trained and tested with a batch size of 32 on one NVIDIA V100 GPU using Stochastic Gradient Descent (SGD) for 30 training epochs.
The taken training time is about 5 hours and 3 hours for ActivityNet Captions and Charades-STA datasets, respectively.
We set hyper-parameters as $\lambda_1=\lambda_2=0.15$, $\beta_1=0.1$, and $\beta_2=0.15$.
Hyper-parameters are chosen by ablations studies.
All hyper-parameters are also described in the configuration files of the provided \path{code} folder.

\begin{figure*}[t]
  \centering
  \includegraphics[width=0.8\linewidth]{figures/6-suppl-different-masks.pdf}
  \caption{
  The shape of different masks:
  (a) a Gaussian mask, (b) a Laplace mask, and (c) an inverse Gaussian mask.
  }
\label{supp-fig:different-masks}
\end{figure*}

%% Variants for ablation studies %%%%%%%%%%%%%%%%%%%%%%%%%%%%%%
\section{Variants for Ablation Studies}
\label{supp-sec:variants-for-ablation-studies}
%%%%%%%%%%%%%%%%%%%%%%%%%%%%%%%%%%%%%%%%%%%%%%%%%%%%%%%%%%%%%

In this section, we elaborate on the variants used for ablation studies.

\subsection{Gaussian generation}
Tab.~{2} shows the impact of different proposal types and strategies for the positive proposal.
In the `Single Gaussian' type of positive proposals, each positive proposal is represented by one Gaussian mask with one learnable width and one learnable center.
Since there is only one mask for one proposal, the `Single Gaussian' type does not use the pulling loss $\mathcal{L}_{pull}$ and the intra-pushing loss $\mathcal{L}^{intra}_{push}$.
The `Gaussian mixture' type of the positive proposals is described in the modeling of GMP for the positive proposal of Sec.~{3}.
For Gaussian generation, we vary how the masks are learned by using three strategies: 1) `Learning one center \& multiple widths', 2) `Learning multiple centers \& widths', and 3) `Learning multiple centers \& one width'.
In `Learning one center \& multiple widths', each proposal $\mathbf{P}_{p}^{(k)}$ has multiple learnable widths and
only one shared learnable center $\mathbf{c}^{(k)} \in \mathbb{R}$ for Gaussian masks.
Since the masks are placed at the same locations, the `Learning one center \& multiple widths' does not use the pulling loss $\mathcal{L}_{pull}$ and the intra-pushing loss $\mathcal{L}^{intra}_{push}$.
In `Learning multiple centers \& widths', each proposal $\mathbf{P}_{p}^{(k)}$ has multiple learnable centers and widths for Gaussian masks as described in Sec.~{3}.
In `Learning multiple centers \& one width', each proposal $\mathbf{P}_{p}^{(k)}$ has multiple learnable centers and only one shared learnable width $\mathbf{s}^{(k)} \in \mathbb{R}$ for Gaussian masks.
For PPS, we adopt the strategy of `Learning multiple centers \& one width', which yields the best performance, as shown in Tab.~{2}.

\subsection{Importance weighting}
In Tab.~{2}, we also use various strategies for mask importance in the Gaussian mixture proposals, where `No importance', `Importance from the generator', and `Importance from the reconstructor' are used.
The strategy of `No importance' generates the $k^{th}$ positive proposals by summing up the Gaussian masks without any importance.
The strategy of `Importance from the generator' estimates mask importance weights through the transformer in the generator.
First, in the Gaussian mixture proposal generation, we replace the original transformer with the MC transformer~\cite{zheng2022cnm}, which is similar to Eq.~({8}), while preserving parameters of the original transformer.
Then, given a video feature $\widehat{\mathbf{V}}$, a sentence query feature $\mathbf{Q}$, and a mask $\mathbf{M}$, we can make a masked multi-modal feature $\mathbf{G}^\mathbf{M}$ which is given by
\begin{equation}
  \mathbf{G}^\mathbf{M}=f_{md}(\widehat{\mathbf{V}}, f_{me}(\mathbf{Q},\mathbf{M}), \mathbf{M}) \in \mathbb{R}^{(T+1)\times d_G} \text{.}
  \label{supp-eq:generative-transformer}
\end{equation}
Here, the MC transformer uses $\mathbf{Q}$ and $\mathbf{M}$ as inputs to the transformer encoder $f_{me}(\cdot)$.
Then, the transformer decoder $f_{md}(\cdot)$ gets $\widehat{\mathbf{V}}$, $f_{me}(\mathbf{Q},\mathbf{M})$, and $\mathbf{M}$. 
$d_G$ is the dimension of the multi-modal feature.
In $\mathbf{G}^\mathbf{M}=[\mathbf{g}^\mathbf{M}_1,\mathbf{g}^\mathbf{M}_2,\dots,\mathbf{g}^\mathbf{M}_{T}, \mathbf{g}^\mathbf{M}_{cls}]^\top$, the vector $\mathbf{g}^\mathbf{M}_{cls}$ is aware of all words and video segments conditioned by the mask $\mathbf{M}$.
To compute the $k^{th}$ mask importance weights $\mathbf{w}^{(k)}$ in Eq.~({4}), we first calculate $\mathbf{g}^{\mathbf{M}_{l}^{(k)}}_{cls}$ using $\mathbf{M}_{l}^{(k)}$ via \cref{supp-eq:generative-transformer} and apply it to a Multi-Layer Perceptron~(MLP) with two layers followed by a Softmax function as follows:
\begin{align}
  &h^{(k)}_l = \mathrm{MLP}\Bigl(\mathbf{g}^{\mathbf{M}_{l}^{(k)}}_{cls}\,\Bigr)\in \mathbb{R} \text{,}
  \label{supp-eq:mask-importance-value-gen} \\
  &\mathbf{w}^{(k)} = \mathrm{Softmax}\Bigl([h^{(k)}_1,h^{(k)}_2,\dots,h^{(k)}_{E_p}]^\top\Bigr) \in\mathbb{R}^{E_p} \text{,}
  \label{supp-eq:mask-importance-weight-gen}
\end{align}
where $E_p$ is the number of masks for the positive proposal.
% We set $E_p$ to $k$ to reflect a varying number of masks in each positive proposal.
The strategy of `Importance from the reconstructor' highlights meaningful masks for query reconstruction in Eq.~({4}) using importance in Eq.~({10}).

\begin{table*}[h]
  \centering
  \resizebox{0.7\linewidth}{!}{
  \begin{tabular}{l c ccc ccc}
    \toprule
    \multirow{2}{*}{Method} & &\multicolumn{3}{c}{Charades, R@1,IoU=0.5} & \multicolumn{3}{c}{ActivityNet, R@1,IoU=0.3} \\ 
    & & iid$^*$ & ood$^*$ &  origin & iid$^*$ & ood$^*$ & origin   \\
    \midrule
    \multirow{5}{*}{Fully supervised} & DRN & 41.91 & 30.43  & 53.09 & 48.92 & 36.86 & - \\
    & SCDM
    & \textbf{47.36} & 41.60 & 54.44  & 46.44 & 31.56 & 54.80 \\
    & LGI
    & - & - & 59.46  & - & - & 58.52\\
    & CBLN
    & - & - & \textbf{61.13}  & - & - & \textbf{66.34}\\
    & MMN
    & - & - & - & - & - & 65.05\\
    \midrule
    \multirow{2}{*}{Weakly supervised} & WS-DEC & 14.06 & 23.67 & - & 26.06 & 17.00 & 41.98  \\
    & PPS (ours) & 46.20 & \textbf{43.18} & 51.49 & \textbf{53.67} & \textbf{41.03}   & 59.29 \\
    \bottomrule
  \end{tabular}}
  \caption{Performance comparisons with fully supervised methods on Charades-STA, Charades-CD, ActivityNet Captions, and ActivityNet-CD datasets. The mark with $^*$ denotes the results on CD dataset and discounted metric in~\cite{yuan2021closer}.}
  % \\
  % \small{$^*$: CD dataset and discounted metric in~\cite{yuan2021closer}.}
  \label{tab:comparisons-CD}
\end{table*}

\begin{table*}[t]
  \centering
          \begin{subtable}[t]{.47\linewidth}
              \centering
              \resizebox{\columnwidth}{!}{
              \begin{tabular}{l c ccc ccc}
                \toprule
                \multirow{2}{*}{Method} & Pre-trained & \multicolumn{3}{c}{R@1}\\ 
                 & features & IoU=0.1 & IoU=0.3 & IoU=0.5 \\
                \midrule
                CNM$^*$ & C3D &79.74 & 54.61 & 30.26 \\
                CNM & CLIP & 78.13 & 55.68 & \underbar{33.33} \\
                \midrule
                PPS (ours) & C3D & \underbar{81.84} & \underbar{59.29} & 31.25 \\
                PPS (ours) & CLIP & \textbf{84.61} & \textbf{62.65} & \textbf{35.80} \\
                \bottomrule
              \end{tabular}}
              \caption{Performance comparisons of using different pre-trained features. The best results and second best results are represented as bold and underlined numbers, respectively. CNM$^*$ is the reproduced CNM using C3D features.} 
              \label{supp-tab:comparisons-activitynet-cnm}
              % \small{CNM$^*$: the reproduced CNM using C3D features.}
            \end{subtable}%
        \hspace{0.2cm}
        \begin{subtable}[t]{.47\linewidth}
            \centering
              \resizebox{\columnwidth}{!}{
              \begin{tabular}{ccc c c}
                \toprule
                \multicolumn{3}{c}{$\mathcal{L}_{rec}$ components} & &\\ 
                Positive & Hard negative & Easy negative & R@1 & R@5 \\
                $C(\mathbf{P}_{p}^{(k^*)})$ & $C(\mathbf{P}_{hn})$ & $C(\mathbf{P}_{en}^{(k^*)})$ & mIoU & mIoU \\
                \midrule
                \cmark & \xmark & \xmark & 27.26 & 56.02 \\
                \xmark & \cmark & \xmark & 35.80 & 52.14 \\
                \xmark & \xmark & \cmark & 25.93 & 53.64 \\
                \xmark & \cmark & \cmark & 34.67 & 50.17 \\
                \cmark & \xmark & \cmark & 27.12 & 52.76 \\
                \cmark & \cmark & \xmark & \textbf{37.59} & \textbf{58.78} \\
                \cmark & \cmark & \cmark & 34.38 & 55.32 \\
                \bottomrule
              \end{tabular}}
              \caption{Performance comparisons by varying components of the reconstruction loss $\mathcal{L}_{rec}$.} 
              \label{supp-tab:ablation-reconstruction-loss}
        \end{subtable}%
        \caption{More experimental results on the ActivityNet Captions dataset.}
  \label{supp-tab:ablation-others2}
\end{table*}

\subsection{Negative proposal mining}
In~\cref{supp-tab:ablation-negative-proposal-types},
we study the impact of different types for the easy negative proposal.
Here, not-learnable masks are defined by positive proposals.
On the contrary, our PPS leverages learnable easy negative proposals.
For ablation studies, we generate the not-learnable easy negative proposals representing the left side and the right side in the video, where confusing temporal locations can be included.
We define one `Not-learnable inverse Gaussian' mask as the $k^{th}$ easy negative proposal to capture both sides of the video, where the center and width are the same as the center and width of the $k^{th}$ positive proposal.
For the `Not-learnable Gaussian' masks, we define two not-learnable Gaussian masks as the $k^{th}$ easy negative proposal to capture both sides of the video.
When the $k^{th}$ positive proposal has the center $c_p$ and the width $w_p$, the widths of the not-learnable Gaussian masks are defined as $w_{en,1}=c_p-w_p/2$ and $w_{en,2}=1-c_p-w_p/2$ and the centers are defined as $c_{en,1}=w_{en,1}/2$ and $c_{en,2}=1-w_{en,2}/2$.
For the `Learnable inverse Gaussian' masks, we define one learnable inverse Gaussian mask $\mathbf{M}_{en}^{(k)}\in \mathbb{R}^{T}$ as the $k^{th}$ easy negative proposal $\mathbf{P}_{en}^{(k)}$, which can be calculated by
\begin{equation}
  \mathbf{M}_{en}^{(k)} = [1-f_{en}^{(k)}(0), 1-f_{en}^{(k)}(1), \dots, 1-f_{en}^{(k)}(T-1)]^\top
  \text{,}
\label{supp-eq:easy-negative-mask2}
\end{equation}
where $f_{en}^{(k)}(\cdot)$ is a Gaussian function for the mask $\mathbf{M}_{en}^{(k)}$, similar to Eq.~({3}).
The shape of the inverse Gaussian mask is depicted in \cref{supp-fig:different-masks}.
The `Learnable Gaussian' masks for the easy negative proposals are defined in the negative proposal mining in Sec.~{3}.

\subsection{Strategies for the pulling loss}
To explore the pulling loss $\mathcal{L}_{pull}$, we perform ablation studies of different strategies for the pulling loss in Tab.~{4b}, which are 1) `Pull all masks', 2) `Pull to the mid', and 3) `Pull distant masks'.
The `Pull all masks' strategy makes all centers of Gaussian masks stay closer, which can be defined as
\begin{equation}
  \mathcal{L}_{pull} = \sum_{k=1}^K\sum_{l_1=1}^{E_p-1}\sum_{l_2=l_1+1}^{E_p} \left(\mathbf{c}^{(k)}_{l_1} - \mathbf{c}^{(k)}_{l_2}\right)^2 \text{.}
  \label{supp-eq:pulling-loss2}
\end{equation}
The `Pull to the mid' strategy brings the centers of the two farthest masks together in the center of the middle mask as follows:
\begin{equation}
  \begin{split}
      \mathcal{L}_{pull} = \sum_{k=1}^K \Bigl(&\bigl(\mathbf{c}^{(k)}_{l_{min}} - \mathbf{c}^{(k)}_{l_{mid}}\bigl)^2 + \\ &\bigl(\mathbf{c}^{(k)}_{l_{max}} - \mathbf{c}^{(k)}_{l_{mid}}\bigl)^2\Bigl) \text{,}
      \label{supp-eq:pulling-loss3}
  \end{split}
\end{equation}
where $l_{min}=\mathrm{arg\,min}_l\, \mathbf{c}^{(k)}_{l}$, $l_{max}=\mathrm{arg\,max}_l\, \mathbf{c}^{(k)}_{l}$, and $l_{mid}$ is the index where $\mathbf{c}^{(k)}_{l_{mid}}$ is the median in $\{\mathbf{c}^{(k)}_{l}\}_{l=1}^k$.
The `Pull distant masks' strategy is defined in the losses for the pull-push learning scheme.

%% More quantitative results %%%%%%%%%%%%%%%%%%%%%%%%%%%%%%
\section{More Quantitative Results}
\label{supp-sec:more-quantitative-results}
%%%%%%%%%%%%%%%%%%%%%%%%%%%%%%%%%%%%%%%%%%%%%%%%%%%%%%%%%%%%%

In this section, we conduct additional quantitative experiments for PPS as follows: 1) comparing performances with fully supervised methods, 2) analyzing moment annotation biases using different splitting strategies, 3) studying the impact of different pre-trained features, 4) studying the impact of different components for the reconstruction loss, 5) studying the effect of leveraging another shape of learnable masks, 6) verifying the effectiveness of training with one proposal, 7) studying the impact of a weight for the intra-video contrastive loss, 8) analyzing the negative proposal mining, 9) studying the impact of a weight for controlling the width of predictions, 10) studying the impact of inference strategies, 11) studying the impact of large proposals, and 12) measuring the inference time and parameters.

\begin{table*}[t]
  \centering
  \resizebox{0.60\linewidth}{!}{
  \begin{tabular}{c c cccc}
    \toprule
    \multirow{2}{*}{Proposal type} & Loss & \multicolumn{2}{c}{R@1} & \multicolumn{2}{c}{R@5} \\ 
      & $\mathcal{L}_{pull}$ \& $\mathcal{L}^{intra}_{push}$ & IoU=0.3 & mIoU & IoU=0.3 & mIoU \\
    \midrule
    Laplace & \xmark & 51.93 & 35.24 & 80.14 & 57.73 \\
    Gaussian & \xmark & 47.49 & 33.33 & 78.23 & 54.85 \\ \midrule
    Laplace mixture & \cmark & 55.76 & 35.09 & 82.49 & \textbf{60.09} \\
    Gaussian mixture & \cmark & \textbf{59.29} & \textbf{37.59} & \textbf{85.54} & 58.78 \\
    \bottomrule
  \end{tabular}}  
  \caption{Performance comparisons of different positive proposals on the ActivityNet Captions dataset.}
  \label{supp-tab:ablation-positive-proposals2}
\end{table*}

\subsection{Comparison with fully supervised methods}
We compare our weakly-supervised PPS with fully supervised temporal video grounding methods:
DRN~\cite{zeng2020dense},
SCDM~\cite{yuan2019semantic},
LGI~\cite{mun2020local},
CBLN~\cite{liu2021context}, and
MMN~\cite{wang2022negative}.
As shown in the results indicated by `origin' in \cref{tab:comparisons-CD}, the results show that our weakly supervised PPS achieves promising results comparable to the fully supervised methods~\cite{zeng2020dense,yuan2019semantic, mun2020local, liu2021context,wang2022negative}.

\subsection{Analysis on moment annotation biases}
To analyze the moment annotation biases, we conducted experiments on CD dataset (iid, ood) and discounted metric in~\cite{yuan2021closer}. 
As shown in the results indicated by $^*$ of \cref{tab:comparisons-CD},
our PPS outperforms the weakly supervised methods (WS-DEC~\cite{duan2018weakly}) and fully supervised methods (DRN~\cite{zeng2020dense},
SCDM~\cite{yuan2019semantic}). 
These results imply that our PPS is less affected by moment annotation biases. In our opinion, the reason is that PPS is trained to reconstruct the query by using Gaussian mixture proposals without using any moment annotations.

\subsection{Impact of different pre-trained features.}
As described in Sec.~{4}, 
some methods use recent large pre-trained features.
Especially, CNM~\cite{zheng2022cnm} uses recent CLIP features~\cite{radford2021learning}.
For a fair comparison, we reproduce the results of CNM with the C3D features~\cite{tran2015learning}, which is denoted as CNM$^*$, using the publicly available code of the CNM\footnote{{https://github.com/minghangz/cnm}.} on the ActivityNet Captions.
Moreover, in PPS, we conduct experiments of replacing the C3D features with CLIP features to study the impact of different pre-trained features.
The results in \cref{supp-tab:comparisons-activitynet-cnm} show that our PPS with C3D outperforms CNM with C3D by margins of $2.1\%$, $4.68\%$, and $0.99\%$ at R@1,IoU=0.1, R@1,IoU=0.3, and R@1,IoU=0.5, respectively.
Also, our PPS with CLIP outperforms CNM with CLIP by large margins of $6.48\%$, $6.97\%$, and $2.47\%$ at R@1,IoU=0.1, R@1,IoU=0.3, and R@1,IoU=0.5, respectively.
Performance improvements at all evaluation metrics show that the generated proposals of PPS promise a higher level of quality.
We only compare the performance at R@1 because CNM is not able to generate multiple proposals while PPS generates multiple proposals.

\begin{figure}[t!]
  \centering
    \begin{subfigure}[b]{\linewidth}
         \centering
         \includegraphics[width=\linewidth]{figures/6-suppl-num-optimized_props.pdf}
         \caption{}
         \label{supp-fig:ablation-graph-num-optim-props}
    \end{subfigure}
    \vfill
    \begin{subfigure}[b]{\linewidth}
         \centering
         \includegraphics[width=\linewidth]{figures/6-suppl-alpha1.pdf}
         \caption{}
         \label{supp-fig:ablation-graph-alpha1}
    \end{subfigure}
    \caption{Ablation studies of varying (a) the number of proposals for training and (b) a $\alpha_1$ value for the intra-video contrastive loss  $\mathcal{L}_{ivc}$ on the ActivityNet Captions dataset.
    % $\alpha$, $\alpha_3$, and $\alpha_4$ for balancing losses
    }
\label{supp-fig:ablation-graph2}
\end{figure}

\subsection{Impact of different components for the reconstruction loss}
In the losses for reconstruction, we use a reconstruction loss, minimizing the cross-entropy losses of
the positive proposals and the hard negative proposal.
In \cref{supp-tab:ablation-reconstruction-loss}, we study the impact of different components for the reconstruction loss $\mathcal{L}_{rec}$.
The results show that minimizing the cross entropy losses of the positive proposal ($C(\mathbf{P}_{p}^{(k^*)})$) and the hard negative proposal ($C(\mathbf{P}_{hn})$) performs best, where query-relevant locations can exist.
On the other hand, minimizing the cross entropy loss of the easy negative proposal ($C(\mathbf{P}_{en})$) degrades performance because the goal of the easy negative proposal is to capture confusing intra-video temporal locations via the intra-video contrastive loss $\mathcal{L}_{ivc}$.

\subsection{Leveraging another shape of learnable masks}
To explore another type of learnable masks, we replace Gaussian masks in Eq.~({3}) with Laplace masks in \cref{supp-eq:laplace} for positive proposals, where the mask function $f_{l}^{(k)}(\cdot)$ is defined as
\begin{equation}
  f_{l}^{(k)}(t) = \mathrm{exp}\left(-\frac{|t/(T-1)-\mathbf{c}^{(k)}_{l}|}{\mathbf{s}^{(k)}_{l}}\right) \text{,} 
  \label{supp-eq:laplace}
\end{equation}
where $\mathbf{c}^{(k)}_{l} \in \mathbb{R}$ and $\mathbf{s}^{(k)}_{l} \in \mathbb{R}$ are the $l^{th}$ elements of $\mathbf{c}^{(k)}$ and $\mathbf{s}^{(k)}$, respectively.
The shape of the Laplace mask is depicted in \cref{supp-fig:different-masks}.
As shown in \cref{supp-tab:ablation-positive-proposals2}, using one Gaussian mask for the positive proposal is less effective than using one Laplace mask.
This is because one Laplace mask can cover a large area in the video and provide a broader view for temporal locations, which has higher values at its tails, as shown in \cref{supp-fig:different-masks}.
On the other hand, using the Gaussian mixture for the positive proposal can make a better performance than using the Laplace mixture.
We conjecture that, due to the sharp shape on its peak, Laplace masks have a worse expression ability for diverse query-relevant events than Gaussian masks.

\paragraph{Future work.}
{We think that masks other than Gaussian or Laplace still can be explored to represent the complex temporal structure.
Besides, the strategies of mixing diverse learnable masks all together can be studied for future work.}

\begin{table*}[t!]
  \centering
\begin{subtable}[t]{.52\linewidth}
  \centering
  \resizebox{\columnwidth}{!}{
  \begin{tabular}{cc cccc}
    \toprule
    \multicolumn{2}{c}{Easy negative proposal} & \multicolumn{2}{c}{R@1} & \multicolumn{2}{c}{R@5} \\ 
    Type & Learnable & IoU=0.3 & mIoU & IoU=0.3 & mIoU \\
    \midrule
    Inverse Gaussian & \xmark & 49.96 & 32.38 & 82.81 & 57.98 \\ 
    Gaussian & \xmark & 45.46 & 33.32 & 79.87 & 56.24 \\ 
    % saturated Gaussian & \xmark & 46.93 & 33.39 & 81.11 & 56.33 \\
    \midrule
    Inverse Gaussian & \cmark & 47.99 & 32.20 & 80.82 & 57.23 \\ 
    Gaussian & \cmark & \textbf{59.29} & \textbf{37.59} & \textbf{85.54} & \textbf{58.78} \\ 
    \bottomrule
  \end{tabular}}
  \caption{Performance comparisons by varying types of easy negative proposals on the ActivityNet Captions dataset.}
  \label{supp-tab:ablation-negative-proposal-types}
\end{subtable}
\hspace{0.7cm}
    \begin{subtable}[t]{.33\linewidth}
        \centering
              \resizebox{\columnwidth}{!}{
              \begin{tabular}{cc cc}
                \toprule
                \multirow{2}{*}{Negative proposal} & \multirow{2}{*}{$\mathcal{L}_{ivc}$} & R@1 & R@5 \\ 
                 &  & mIoU & mIoU \\
                \midrule
                None & \xmark & 31.44 & 53.08 \\ 
                Only hard & \cmark & 32.49 & 56.23 \\ 
                Only easy & \cmark & 30.75 & 57.21 \\ 
                Both hard \& easy & \cmark & \textbf{37.59} & \textbf{58.78} \\ 
                \bottomrule
          \end{tabular}}
          \caption{Ablation studies of hard \& easy negative proposals.}
          \label{supp-tab:ablation-negative-proposal-loss}
  \end{subtable}
    \caption{Ablation study on negative proposal mining of PPS on the ActivityNet Captions dataset.}
  \label{supp-tab:ablation-others4}
\end{table*}

\begin{table*}[t!]
  \centering
   \begin{subtable}[t]{.26\linewidth}
            \centering
              \resizebox{\columnwidth}{!}{
              \begin{tabular}{c cc}
                \toprule
                {Easy negative} & R@1 & R@5 \\ 
                Proposal & mIoU & mIoU \\
                \midrule
                None & \textbf{37.59} & \textbf{58.78}\\
                Varying num & 35.89 & 56.19 \\ 
                importance & 34.59 & 57.28 \\ 
                Pull-push & 34.36 & 57.25 \\ 
                \bottomrule
            \end{tabular}}
              \caption{Performance comparisons by varying strategies for the easy negative proposals}
              \label{supp-tab:ablation-negative-proposals}
        \end{subtable}%
        \hspace{0.7cm}
        \begin{subtable}[t]{.20\linewidth}
        \centering
          \resizebox{\columnwidth}{!}{
          \begin{tabular}{c cc}
            \toprule
            \multirow{2}{*}{$\gamma$} & R@1 & R@5 \\ 
             & mIoU & mIoU \\ \midrule
            1 & 37.05 & 58.80 \\ 
            0.95 & 37.44 & \textbf{58.85} \\ 
            0.9 & 37.58 & \textbf{58.85} \\ 
            0.85 & \textbf{37.59} & 58.78 \\ 
            0.8 & 37.50 & 58.66 \\ 
            0.75 & 37.28 & 58.47 \\ 
            \bottomrule
      \end{tabular}}
      \caption{Performance comparisons by varying $\gamma$ for inference.}
      \label{supp-tab:ablation-inference-gamma}
  \end{subtable}
    \hspace{0.7cm}
    \begin{subtable}[t]{.24\linewidth}
        \centering
          \resizebox{\columnwidth}{!}{
          \begin{tabular}{c cc}
            \toprule
            Inference & R@1 & R@5 \\ 
            strategy & mIoU & mIoU \\
            \midrule
            Tail-to-tail & 36.09 & 55.23 \\ 
            Average & 37.24 & 57.63 \\
            Importance & \textbf{37.59} & \textbf{58.78} \\
            \bottomrule
      \end{tabular}}
      \caption{Performance comparisons of different inference strategies.}
      \label{supp-tab:ablation-inference}
    \end{subtable}%
    \caption{Ablation study on different strategies of PPS on the ActivityNet Captions dataset.}
  \label{supp-tab:ablation-others3}
\end{table*}

\subsection{Training with multiple proposals}
To focus on the most query-relevant proposal, we only exploit the positive proposal $\mathbf{P}_p^{(k^*)}$ in the losses for reconstruction, where $k^* = \mathrm{arg\,min}_k\,C(\mathbf{P}_{p}^{(k)})$.
To verify the effectiveness of this exploitation, we compare the results by varying the number of proposals for training in \cref{supp-fig:ablation-graph-num-optim-props}.
When the number of proposals for training is $n_{opt}$, we select the $n_{opt}$ proposals with the lowest cross-entropy losses $C(\mathbf{P}_{p}^{(k)})$ for the reconstruction loss.
The results show that training fewer proposals perform better than training more proposals.
We conjecture that training one proposal with the minimum cross-entropy loss helps each proposal to specialize in different contexts in a video and a query, which can be considered as similar results in the multiple choice learning~\cite{guzman2012multiple}.

\subsection{Impact of a weight for the intra-video contrastive loss}
\cref{supp-fig:ablation-graph-alpha1}
shows the impact of controlling $\alpha_1$ for the intra-video contrastive loss $\mathcal{L}_{ivc}$.
The performance increases until the number is $1$ and decreases after it.
This result suggests that an adequate $\alpha_1$ value for $\mathcal{L}_{ivc}$ is needed to perform effective contrastive learning that distinguishes Gaussian mixture proposals (positive) from confusing intra-video temporal locations (negative).

% is needed to make densely generated masks and adequate $\alpha$ values for the pushing losses are needed to give proper discrimination between the masks and the proposals.

\subsection{Analysis of negative proposal mining.}
As shown in \cref{supp-tab:ablation-negative-proposal-types}, we study the impact of different types for the easy negative proposal.
Not-learnable masks are only defined by positive proposals.
The proposed learnable Gaussian masks are more effective as they capture confusing locations throughout the entire video.
Further, the learnable inverse Gaussian masks meant to cover a large area in the video are less effective.
The results suggest that capturing small but highly confusing locations is important for contrastive learning.
Moreover, we verify the effectiveness of hard and easy negative proposals in \cref{supp-tab:ablation-negative-proposal-loss}.
Especially, using both easy and hard negative proposals can improve performance by capturing diverse and highly confusing locations.
Fig.~{3} shows the impact of the number of masks $E_{en}$ for each easy negative proposal.
The performance increases until the number is $2$ and $4$ at R@1 and R@5, respectively.
The results imply that multiple learnable masks for a negative proposal are needed to capture diverse confusing locations that are helpful for contrastive learning.
% , but, if the number is too large, it may spoil the contrastive learning.

% \subsection{Analysis on the strategies for the easy negative proposals}
\cref{supp-tab:ablation-negative-proposals} presents the diverse strategies for generating the easy negative proposals, which are composed of `Varying num', `Importance', and `Pull-push' which are strategies used for positive proposal generation.
For `Varying num', we set the number of masks $E_{en}$ to $k$ in the $k^{th}$ easy negative proposal for reflecting a varying number of masks in each proposal.
For `Importance', we apply mask importance to the masks in the easy negative proposals, using the similar process in Eq.~({8}) to ({10}).
By using the mask importance, we can reflect reconstruction-aware information in the easy negative proposals.
For `Pull-push', we apply the equivalent pull-push learning scheme, which is only used for the positive proposals, to the easy negative proposals.
The pull-push learning scheme uses a pulling loss in Eq.~({5}) and two pushing losses in Eq.~({6}) and ({7}), each of which plays an opposite role to the other, to produce densely generated and less overlapped masks.
By this learning scheme, the Gaussian masks in each easy negative proposal become moderately coupled.

In \cref{supp-tab:ablation-negative-proposals}, the results are summarized as follows:
First, the `Varying num' strategy reduces performance, showing that combinations of various numbers of masks are not effective.
We conjecture that a fixed number of masks ($E_{en}=2$) can capture small but highly confusing temporal locations, which is important for contrastive learning.
Second, the `Importance' strategy is not effective because importance weights represent importance levels for query relevance and the easy negative proposals aim to capture only confusing locations which are not relevant to the query.
Third, the `Pull-push' strategy degrades performance, which is similar to the result using one mask ($E_{en}=1$) in Fig.~{3} because the masks in each negative proposal are densely generated.
This result implies that letting the masks for each easy negative proposal spread sparsely without the pull-push learning scheme is effective, because multiple confusing temporal locations in a video exist throughout the entire video.

\subsection{Impact of weight for controlling the width of predictions}
We observe that the lengths of the positive proposal and the predicted temporal location do not match well.
Since the tails in the positive proposal have low attention, it is not ideal to use the same width for the positive proposal and the predicted temporal location.
Therefore, we introduce a hyper-parameter $\gamma$ to control the lengths of the predicted temporal locations as shown in \cref{supp-eq:start,supp-eq:end}.
We verify the effect of $\gamma$ in \cref{supp-tab:ablation-inference-gamma}, which shows that setting $\gamma$ to $0.85$ makes slightly a better performance at R@1 for the ActivityNet Captions dataset.
We also set $\gamma$ to $1$ for the Charades-STA dataset.

\begin{figure*}[t!]
  \centering
  \includegraphics[width=0.7\linewidth]{figures/6-more-qualitative.pdf}
  \caption{
  More qualitative results. Given an untrimmed video and a sentence query, we visualize the ground-truth temporal location (grey), the selected positive proposal (purple) with Gaussian masks, the predicted temporal location (red), and the easy negative proposal (blue).
  % Here, darker boxes mean higher values in the corresponding temporal locations.
  }
\label{supp-fig:more-qualitative}
\end{figure*}

\begin{figure*}[t!]
  \centering
  \includegraphics[width=0.74\linewidth]{figures/6-more-qualitative-cpl.pdf}
  \caption{
  Qualitative comparisons with CPL. Given an untrimmed video and a sentence query, we visualize the ground-truth temporal location (brown), the predicted temporal locations of PPS (red), and the predicted temporal locations of CPL (blue).
  PPS and CPL produce the five predicted temporal locations, respectively.
  The top-1 predicted temporal location to the top-5 is depicted from top to bottom.
  }
\label{supp-fig:more-qualitative-cpl}
\end{figure*}

\begin{figure*}[t!]
  \centering
  \includegraphics[width=0.76\linewidth]{figures/6-more-qualitative-pullpush.pdf}
  \caption{
  Qualitative results of PPS without pulling or pushing losses.
  Given an untrimmed video and a sentence query, we visualize the ground-truth temporal location (brown) and the positive proposals (dark boxes) of PPS without the pulling loss and PPS without the pushing loss, respectively.
  PPS generates five positive proposals.
  Here, darker boxes mean higher values in the corresponding temporal locations.
  }
\label{supp-fig:more-qualitative-pullpush}
\end{figure*}

\subsection{Impact of inference strategies}
\cref{supp-tab:ablation-inference} shows the impact of different inference strategies.
Importance-based inference achieves the best performance among the three inference strategies, which predicts temporal locations highlighted by the importance of the masks. 
On the other hand, we observe that tail-to-tail-based inference predicts long temporal locations that yield worse performance.
% Average-based inference shows comparable results with attention-based inference.
% Since averaging can be considered as summing up with equal attention, 
% we conjecture that 
% average-based inference and attention-based inference produce similar results in well-generated masks having similar mask attention weights.

\begin{table}[t]
  \centering
  \resizebox{\columnwidth}{!}{
  \begin{tabular}{l ccc ccc}
    \toprule
    \multirow{2}{*}{$\alpha_{4}$} & \multicolumn{2}{c}{R@1} & \multicolumn{2}{c}{R@5} & \multicolumn{2}{c}{\textbf{R@10}} \\ 
    & IoU=0.5 & mIoU & IoU=0.5 & mIoU & \textbf{IoU=0.5} & \textbf{mIoU}   \\
    \midrule
    0.15 & 26.87 & 29.02 & 48.78 & 47.58 & 73.04 & 61.51 \\
    0.1$^*$ & 27.46 & 29.94 & 54.18 & 50.13 & 76.21 & 62.42 \\
    0.05 & 27.98 & 33.16 & \textbf{57.34} & \textbf{52.69} & \textbf{80.58} & \textbf{67.13}  \\
    0.01 & \textbf{28.65} & \textbf{33.45} & 55.59 & 52.13 & 78.88 & 65.84 \\
    0 & 25.94 & 27.47 & 52.95 & 49.91 & 71.85 & 62.05 \\
    \bottomrule
  \end{tabular}}
  \caption{Performance comparisons of different $\alpha_{4}$ for large proposals on ActivityNet Captions dataset. The used value in our method is denoted as $^*$.}
  % \\ \small{$^*$: value used in the paper.}
  \label{tab:ablation_many_proposals}
\end{table}

\begin{table}[t]
  \centering
  \resizebox{0.88\columnwidth}{!}{
  \begin{tabular}{l cc}
    \toprule
    & Parameters (M) & Inference time (msec) \\
    \midrule
    CNM & 7 & 56 \\
    CPL & 7 & 81 \\
    LoGAN & 11 & - \\
    TGA & 19 &  83\\
    \midrule
    PPS (Ours) & 15 & 92 \\
    \bottomrule
  \end{tabular}}
  \caption{Comparisons of the inference time and parameters on Charades-STA dataset.}
  \label{tab:inference_time_parameters}
\end{table}

%% Analysis on large proposals%%%%%%%%%%%%%%%%%%%%%%%%%%%%%%
\subsection{Analysis on large proposals}
\label{supp-sec:analysis-on-large-proposals}
%%%%%%%%%%%%%%%%%%%%%%%%%%%%%%%%%%%%%%%%%%%%%%%%%%%%%%%%%%%%%
Fig.~{3} shows that accuracy decreases with large proposals.
The decrease is due to the effect of inter-pushing loss $\mathcal{L}^{inter}_{push}$, which pushes proposals away from each other.
If too many proposals try to avoid overlapping of proposals, each proposal tends to capture a small-sized temporal location.
To evaluate the effect of the weight $\alpha_{4}$ of $\mathcal{L}^{inter}_{push}$ for a large number of proposals \textit{K}=10, we have conducted an experiment on R@10 as well as R@1 and R@5.
As shown in \cref{tab:ablation_many_proposals}, the case of $\alpha_{4}$=0.05 performs relatively well even with a large number of proposals (80.58\% and 67.13\% at R@10,0.5 and R@10,mIoU).

%% Comparisons of the inference time and parameters %%%%%%%%%%%%%%%%%%%%%%%%%%%%%%
\subsection{Comparisons of the inference time and parameters}
\label{supp-sec:comparisons_of_the_inference_time_and_parameters}
%%%%%%%%%%%%%%%%%%%%%%%%%%%%%%%%%%%%%%%%%%%%%%%%%%%%%%%%%%%%%
As shown in \cref{tab:inference_time_parameters}, we compare the number of parameters and average inference time of our PPS with other weakly supervised temporal video grounding methods: CNM~\cite{zheng2022cnm},
CPL~\cite{zheng2022cpl},
LoGAN~\cite{tan2021logan}, and
TGA~\cite{mithun2019weakly}.
Our PPS requires 15M parameters and has a comparable speed (92 milliseconds).

%% More qualitative results %%%%%%%%%%%%%%%%%%%%%%%%%%%%%%
\section{More Qualitative Results}
\label{supp-sec:more-qualitative-results}
%%%%%%%%%%%%%%%%%%%%%%%%%%%%%%%%%%%%%%%%%%%%%%%%%%%%%%%%%%%%%
In this section, we illustrate additional qualitative experimental results for PPS as follows: 1) visualization of positive proposals, easy negative proposals, and predicted temporal locations, 2) qualitative comparisons with a single Gaussian proposal, and 3) studying the impact of a pull-push learning scheme.

\subsection{Visualization of proposals}
More qualitative results on both ActivityNet Captions and Charades-STA datasets are depicted in \cref{supp-fig:more-qualitative}.
For each qualitative result, we visualize an untrimmed video and a sentence query, the ground-truth temporal location, the selected positive proposal $\mathbf{P}_{p}^{(k^\dagger)}$ with Gaussian masks, the predicted temporal location from $\mathbf{P}_{p}^{(k^\dagger)}$, and the easy negative proposal $\mathbf{P}_{en}^{(k^\dagger)}$.
The positive proposals capture the temporal locations described by the sentence query while the negative proposals capture the confusing temporal locations.
The predicted temporal locations from the positive proposals are well matched with the ground-truth temporal locations, which means that our PPS solves the problem of weakly supervised temporal video grounding successfully.

% \subsection{Impact of learnable negative proposals}
% In previous methods, negative proposals are defined by subtracting the positive proposals from one~\cite{zheng2022cnm} or making masks outside the positive proposals~\cite{zheng2022cpl}, which are rule-based.
% These rule-based negative proposals are designed to exist outside the positive proposals.
% Therefore, the rule-based negative proposals do not have the ability to capture all confusing temporal locations, because the confusing temporal locations also exist inside poorly generated positive proposals whose quality is low.
% This limitation can accumulate errors as pointed out in~\cite{zheng2022cnm}.
% Unlike the rule-based negative proposals, we leverage multiple learnable Gaussian masks for negative proposals to capture diversely-shaped confusing temporal locations throughout the entire video, as described in the negative proposal mining of Sec.~{3}.
% It is notable that the second and fourth qualitative results in \cref{supp-fig:more-qualitative} have easy negative proposals overlapped with the positive proposals, capturing temporal locations that are less relevant to the query.
% These results suggest that our PPS can learn to capture highly confusing temporal locations even inside the positive proposals.
% We also conjecture that, by leveraging the learnable negative proposals, we can mitigate accumulated errors of the proposal-based reconstructor, which are caused by poorly generated positive proposals during early training.

\subsection{Comparisons with a single Gaussian proposal}
For qualitative comparisons with the method using a single Gaussian proposal, CPL~\cite{zheng2022cpl}, we use the publicly available code of the CPL\footnote{{https://github.com/minghangz/cpl}.} on the ActivityNet Captions.
In \cref{supp-fig:more-qualitative-cpl}, we visualize a sentence query, the ground-truth temporal location, and the predicted temporal locations of PPS and CPL, respectively, where the five predicted temporal locations are produced.
The top-1 predicted temporal location to the top-5 is depicted from top to bottom.
The results show that PPS predicts a more accurate top-1 temporal location than CPL.
Furthermore, PPS can generate temporal locations with various lengths while CPL generates temporal locations with similar lengths that lack the ability to express diverse temporal structures.
Since a single Gaussian mask is a pre-determined shape with a high value at its center, it is not suitable for expressing diverse query-relevant events.
On the contrary, our Gaussian mixture proposals can effectively represent the diverse events, by leveraging multiple learnable Gaussian masks, reconstruction-aware mask importance, and a pull-push learning scheme.

\subsection{Impact of the pull-push learning scheme}
In our scheme, the Gaussian masks in one positive proposal should be densely located near the query-relevant temporal location but should not be overlapped too much with each other to represent proper temporal locations for video grounding.
To this end, we propose a pull-push learning scheme using a pulling loss and a pushing loss, each of which plays an opposite role to the other, to produce densely generated and less overlapped masks.
In \cref{supp-fig:more-qualitative-pullpush},
we visualize a sentence query, the ground-truth temporal location, and the five positive proposals of PPS without the pulling loss and PPS without the pushing loss, respectively.
The results show that PPS without the pulling loss makes the masks spread sparsely throughout the entire video and PPS without the pushing loss makes the proposals overlap at similar locations.
To produce densely generated and less overlapped masks, PPS needs to be trained with a pull-push learning scheme, which leads to significant performance improvements as shown in Tab.~{5}.
However, it is notable that PPS without the pulling or pushing loss still can generate query-relevant temporal locations that have higher values inside the ground-truth temporal location. 

\vspace{1cm}
\noindent
\textbf{\textit{`Code for reproducibility' is continued on the next page.}
}

\vfill\eject
\clearpage

\onecolumn
%% Code for reproducibility %%%%%%%%%%%%%%%%%%%%%%%%%%%%%%
\section{Code for Reproducibility}
\label{supp-sec:code-for-reproducibility}
%%%%%%%%%%%%%%%%%%%%%%%%%%%%%%%%%%%%%%%%%%%%%%%%%%%%%%%%%%%%%

For the reproducibility of our PPS, we provide the specification of dependencies, training codes, evaluation codes, and a README file in the \path{code} folder from the supplementary material ZIP file.
% For the reproducibility of our PPS, we provide the specification of dependencies, training codes, evaluation codes, pre-trained models, and a README file in the \path{code} folder from the supplementary material ZIP file.
This section includes a table of results and precise commands to run to reproduce the results on both the ActivityNet Captions~\cite{krishna2017dense} and Charades-STA~\cite{gao2017tall} datasets. 
The README file contains the same description below.

\subsection{Results}

\begin{table*}[h]
  \centering
          \begin{subtable}[t]{0.8\linewidth}
              \centering
              \resizebox{\linewidth}{!}{
              \begin{tabular}{c cccc cccc}
                \toprule
                 &\multicolumn{4}{c}{R@1} & \multicolumn{4}{c}{R@5} \\ 
                 Method & IoU=0.1 & IoU=0.3 & IoU=0.5 & mIoU & IoU=0.1 & IoU=0.3 & IoU=0.5 & mIoU \\
                \midrule
                PPS (ours) & 81.84 & 59.29 & 31.25 & 37.59 & 95.28 & 85.54 & 71.32 & 58.78 \\
                \bottomrule
              \end{tabular}}
              \caption{Results of PPS on the ActivityNet Captions dataset.}
              \label{supp-tab:PPS-result-activitynet}
            \end{subtable}%
        \hspace{0.2cm}
        \begin{subtable}[t]{0.8\linewidth}
            \centering
              \resizebox{\linewidth}{!}{
              \begin{tabular}{c cccc cccc}
                \toprule
                 &\multicolumn{4}{c}{R@1} & \multicolumn{4}{c}{R@5} \\ 
                 Method & IoU=0.3 & IoU=0.5 & IoU=0.7 & mIoU & IoU=0.3 & IoU=0.5 & IoU=0.7 & mIoU \\
                \midrule
                PPS (ours) & 69.06 & 51.49 & 26.16 & 45.84 & 99.18 & 86.23 & 53.01 & 69.19 \\
                \bottomrule
              \end{tabular}}
              \caption{Results of PPS on the Charades-STA dataset.}
              \label{supp-tab:PPS-result-charades}
        \end{subtable}%
        \caption{Results of PPS.}
  \label{supp-tab:PPS-result}
\end{table*}

\noindent
\cref{supp-tab:PPS-result} shows the results of PPS on both the ActivityNet Captions and Charades-STA datasets.

\subsection{Dependencies}

\noindent
Please use {the NVIDIA PyTorch Container version 21.11}. 
In other versions, the results of our PPS may not be properly reproduced due to the different operations of modules.
The NVIDIA PyTorch image can be pulled using the following command.

{
\begin{lstlisting}[language=bash]
  $ docker pull nvcr.io/nvidia/pytorch:21.11-py3
\end{lstlisting}
}

\noindent
We use the following dependencies for implementation.

\begin{itemize}

\item ubuntu 20.04
\item cuda 11.5
\item python 3.8.12
\item pytorch 1.11.0a0+b6df043 (Not pytorch 1.11.0)
\item nltk 3.4.5
\item wandb 0.12.20
\item h5py 3.7.0
\item fairseq 0.12.2
\end{itemize}

\noindent
If the fairseq automatically installs another version of PyTorch, delete that PyTorch because we use PyTorch version 1.11.0a0+b6df043 (it's not version 1.11.0).

\noindent
Please use the following command to download some resources from the Natural Language Toolkit (nltk).

{
\begin{lstlisting}[language=bash]
  $ python
  >>> import nltk
  >>> nltk.download('punkt')
  >>> nltk.download('averaged_perceptron_tagger')
\end{lstlisting}
}

\subsection{Data preparation}

\noindent
We use two public datasets: the ActivityNet Captions dataset and the Charades-STA dataset.

\noindent
For the ActivityNet Captions dataset,
{C3D} features~\cite{tran2015learning} are used.
We use the converted C3D features provided by {LGI}~\cite{mun2020local}.
Please download the converted C3D features and save them as \path{data/activitynet/sub_activitynet_v1-3.c3d.hdf5}.

\noindent
For the Charades-STA dataset, {I3D}~\cite{carreira2017quo} features are used.
We use the converted I3D features provided by {CPL}~\cite{zheng2022cpl}.
Please download the converted I3D features and save them as \path{data/charades/i3d_features.hdf5}.

\noindent
The directory structure should be

\path{data}

├── \path{activitynet}

│\qquad├── \path{asub_activitynet_v1-3.c3d.hdf5}

│\qquad├── \path{glove.pkl}

│\qquad├── \path{train_data.json}

│\qquad├── \path{test_data.json}

├── \path{charades}

│\qquad├── \path{i3d_features.hdf5}

│\qquad├── \path{glove.pkl}

│\qquad├── \path{train.json}

│\qquad├── \path{test.json}

\subsection{Evaluation of pre-trained models}

\noindent
Here, we describe how to run our implemented codes.

\noindent
We provide our trained models in the folder \path{checkpoint/}.
Due to the limited capacity of the supplementary material (50MB), we will release the trained models later on GitHub, whose size is 64MB and 57MB for ActivityNet Captions and Charades-STA
, respectively.
% \textbf{Due to the limited capacity of the supplementary material (100MB), we only provide the trained model on ActivityNet Captions dataset.
% Other models will be released on GitHub.}

\noindent
For evaluation on the ActivityNet Captions dataset, please use the following command.

\begin{lstlisting}[language=bash]
  $ bash script/eval_activitynet.sh
\end{lstlisting}

% \noindent
For evaluation on the Charades-STA dataset, please use the following command.

\begin{lstlisting}[language=bash]
  $ bash script/eval_charades.sh
\end{lstlisting}

\noindent
Logs and checkpoints are automatically saved in the folders \path{log/} and \path{checkpoint/}, respectively.

\noindent
We use {Wandb} for the visualization of learning curves.
If you want to disable it, please set \path{use_wandb} to \path{False} in the folder \path{config/}.
Also, other configurations can be modified in the folder \path{config/}.

\subsection{Training from scratch}

\noindent
For training the model from scratch on the ActivityNet Captions dataset, please use the following command.

\begin{lstlisting}[language=bash]
  $ bash script/train_activitynet.sh
\end{lstlisting}

\noindent
For training the model from scratch on the Charades-STA dataset, please use the following command.

\begin{lstlisting}[language=bash]
  $ bash script/train_charades.sh
\end{lstlisting}

% \subsection{Repository reference}

% \noindent
% The following repositories were helpful for our implementation.

% {https://github.com/JonghwanMun/LGI4temporalgrounding}

% {https://github.com/minghangz/cpl}

% {https://github.com/jadore801120/attention-is-all-you-need-pytorch}

% {https://github.com/wengong-jin/fairseq-py/tree/master/fairseq/optim}

\noindent

\subsection{GitHub}
Our code will be publicly available on GitHub.

\twocolumn
